# Supplementary material for: Matching with multiple criteria and its application to health disparities research
Source: arXiv:2308.08217 source file (2023-08-16)
Supplement: Supplementary file 1 [file appendix.tex]

\subsection*{A. Additional literature review}
Despite the advantage of network flow optimization in finding the global minimum covariate distance between treated and matched comparisons, conducting such optimization in some large administrative datasets (e.g., the BRFSS database in the motivating example) can become computationally challenging in dense networks, characterized by two disjoint sets of nodes where each node in the first set is connected to every node in the second set. For example, optimally pairing $T$ = 2,507 black male patients with 2,507 white male patients from a pool of $C$ = 23,344 white male patients would require a time complexity of order $O(T^3)$\citep{yu2020matching}. 
\citet{yu2020matching} proposed an approach to enhance the dense matching efficiency and sparse matching feasibility with an iterative variant of Glover's algorithm \citep{glover1967maximum, lipski1981efficient}. This approach uses binary search to find the minimum caliper size that satisfies pair-matching feasibility in a doubly convex bipartite graph with time complexity in the order of $O(T)$. As a result, this approach significantly reduced the pool of potential matches, improving efficiency in constructing optimally matched comparisons with the time complexity of order $O(T^2 \log T)$. Additionally, this approach mitigated infeasibility risk, where a control subject could not be matched with a treated subject.
In addition to the computational challenges of constructing matched comparisons in large datasets, there are also inherent challenges associated with matching based on a nominal covariate with many categories. The process of exact matching on a multi-level covariate becomes increasingly difficult as the number of covariate level increases, due to the exponential growth in the number of possible combinations. Matching based on propensity score can help to balance a large number of covariates, but this method can only achieve stochastic balance. \todo[inline]{Given the shift in our focus of the article, suggest move the latter part of this paragraph, e.g., large data, exact matching, fine balance, etc, to the supplement.}\citet{rosenbaum2007minimum} proposed a matching approach called fine balance which exactly balances the marginal distribution of one nominal variable, often one with many categories, or the joint distribution of several nominal variables between the treated and control units without matching individuals on these covariates. As the fine balance is not always achievable if the controls are always fewer at one level for some covariates, the near-fine balance approach is then implemented with relaxed constraints, aiming to minimize the total absolute difference in frequencies over the categories \citep{yang2012optimal}. As an extension to achieve fine balance on multiple nominal covariates, \citet{pimentel2015large} introduced refined balance to impose a nested, hierarchical structure on observed covariates which prioritizes near-fine balancing on important variables over others \citep{pimentel2015large}.
